# Supplementary material for: Characterizing the greater-than-bulk melting behaviour of Ga-Al nanoalloys
Source: arXiv:1503.03629 source file (2015-03-21)
Supplement: Supplementary file 1 [file SupplementaryInformation.pdf]

# Supporting Information

## 1. Average Coordination Number

An atom is considered a neighbour in the average coordination number calculations if it is at a distance of less-than-or-equal-to 3.6 Å and 3.7 Å in $Ga_{11}Al_9^+$ and $Ga_3Al_{17}^+$ respectively. Fig. 1 shows the changes in the average coordination number of the internal (red and blue) and some representative surface atoms. At all temperatures below the melting temperature of 824 K, the internal Al atoms of $Ga_{11}Al_9^+$ cluster maintain a coordination state of 9 and above. However, after the melting temperature (at the highest energy), the internal and the surface Al atoms still occupy sites with 6.9 to 8.9 neighbouring atoms on average. The surface gallium atoms prefer to stay at the surface at all temperatures.

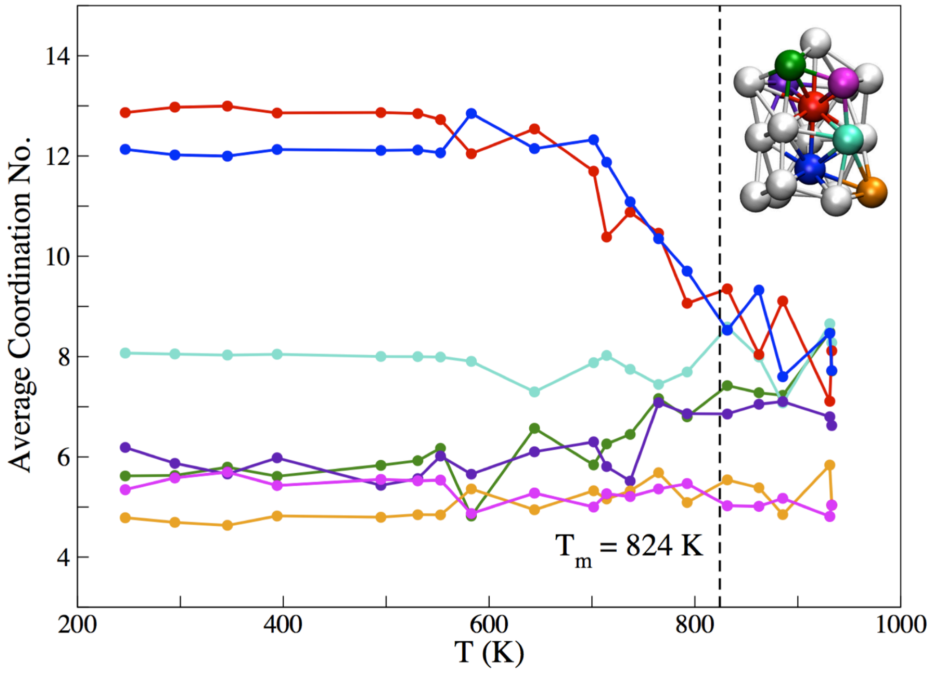


Fig. 1 Average coordination number of representative atoms (coloured in inset) of $Ga_{11}Al_9^+$ cluster

Shown in Fig. 2 is the average coordination number of representative atoms (coloured in inset) of $Ga_3Al_{17}^+$ cluster. Similar to $Ga_{11}Al_9^+$, there is clear difference between the internal Al atoms and the surface Al and Ga atoms in the average coordination number. However, at 778 K (still much below the melting temperature of 922 K) one of the internal atoms (coloured red) comes occupies a coordination site of 9 atoms on average, shoots back up to being an internal atom at the next simulated microcanonical energy (average temperature of 808 K) and comes back down to being a surface atom at 834 K. Furthermore, at 891 K both the lowest energy internal Al atoms (red and blue) are replaced by lowest energy surface Al atoms (magenta and green) which shows the swapping of positions as also confirmed by MD movies. After the melting temperature, at the highest

energy, all the Al atoms are coordinated by 6 to 7 atoms on average and the Ga atoms preferring the low coordinated surface sites.

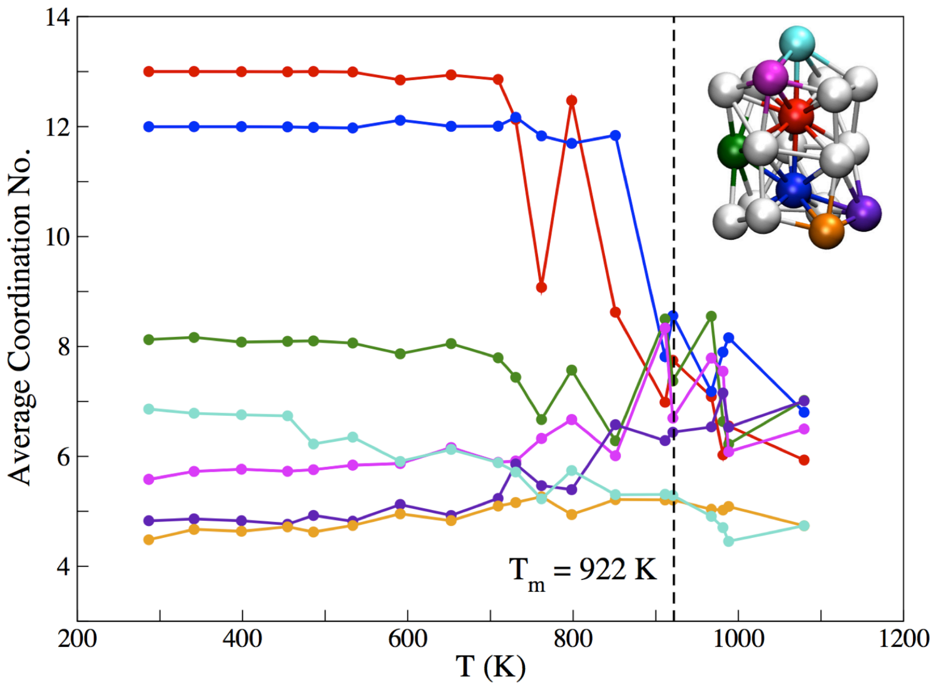


Fig. 2 Average coordination number of representative atoms (coloured in inset) of $Ga_3Al_{17}^+$ cluster.

## 2. Bader Charges

Fig. 3 shows the partial charges associated with Ga and Al atoms using the atoms-in-molecules analysis.  In both clusters we observe strong charge segregation between the internal and surface atoms. The more highly coordinated internal Al atom gets negatively charged and the other internal Al atom stays neutral in both cases. Moreover, among the surface atoms, it is the Ga atom that gets either negatively charged or stays neutral and the Al atoms are either positively charged or neutral.

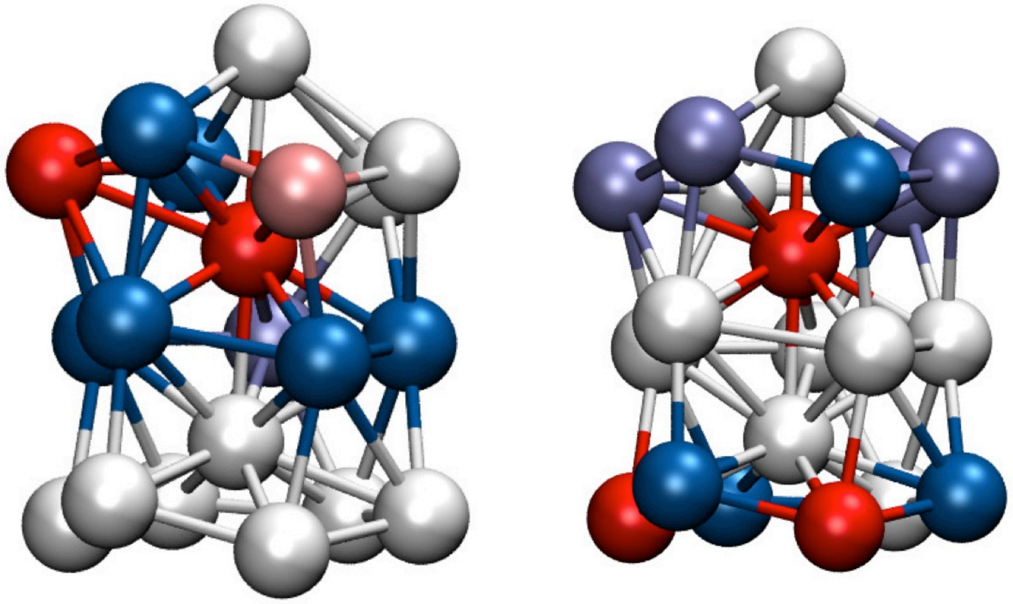

(a) $Ga_{11}Al_9^+$ (b) $Ga_3Al_{17}^+$

Fig. 3 Partial charges (q) obtained by atoms in molecules (AIM) analysis: (red) q ≤ -0.2e; (pink) -0.2e < q ≤ -0.1e; (white) -0.1e < q ≤ 0.1e; (ice blue) 0.1e < q ≤ 0.2e; (dark blue) q > 0.2e.

## 3. Exchange between Internal and external atoms and sites

All the structures shown have been snapped from MD movies at 809 K of $Al_{20}^{+}$ cluster using VMD[1] software. All the atoms have been coloured differently to bring out the difference in the sites.

[1] Humphrey, W., Dalke, A. and Schulten, K., "VMD - Visual Molecular Dynamics", J. Molec. Graphics, 1996, vol. 14, pp. 33-38.

(a) Due to parallel tempering:

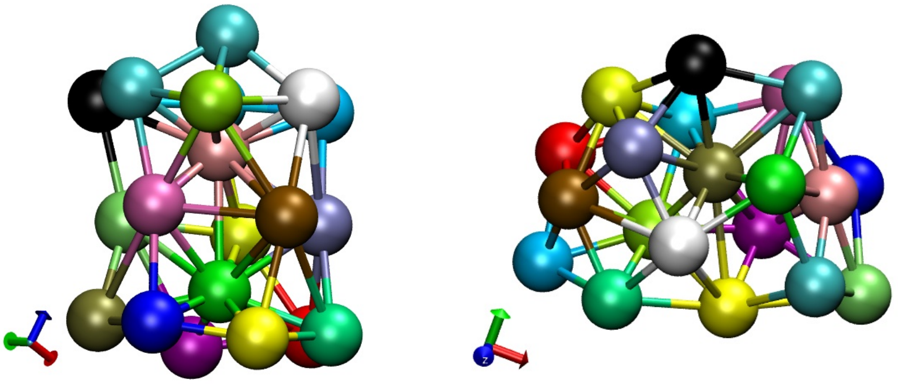

Fig. 4 Changes in the structure and the number and atom occupying the internal site due to parallel tempering as observed in the movie. This happens between 9.800 and 9.801 ps.

(b) Stage-wise change in the number of internal atoms

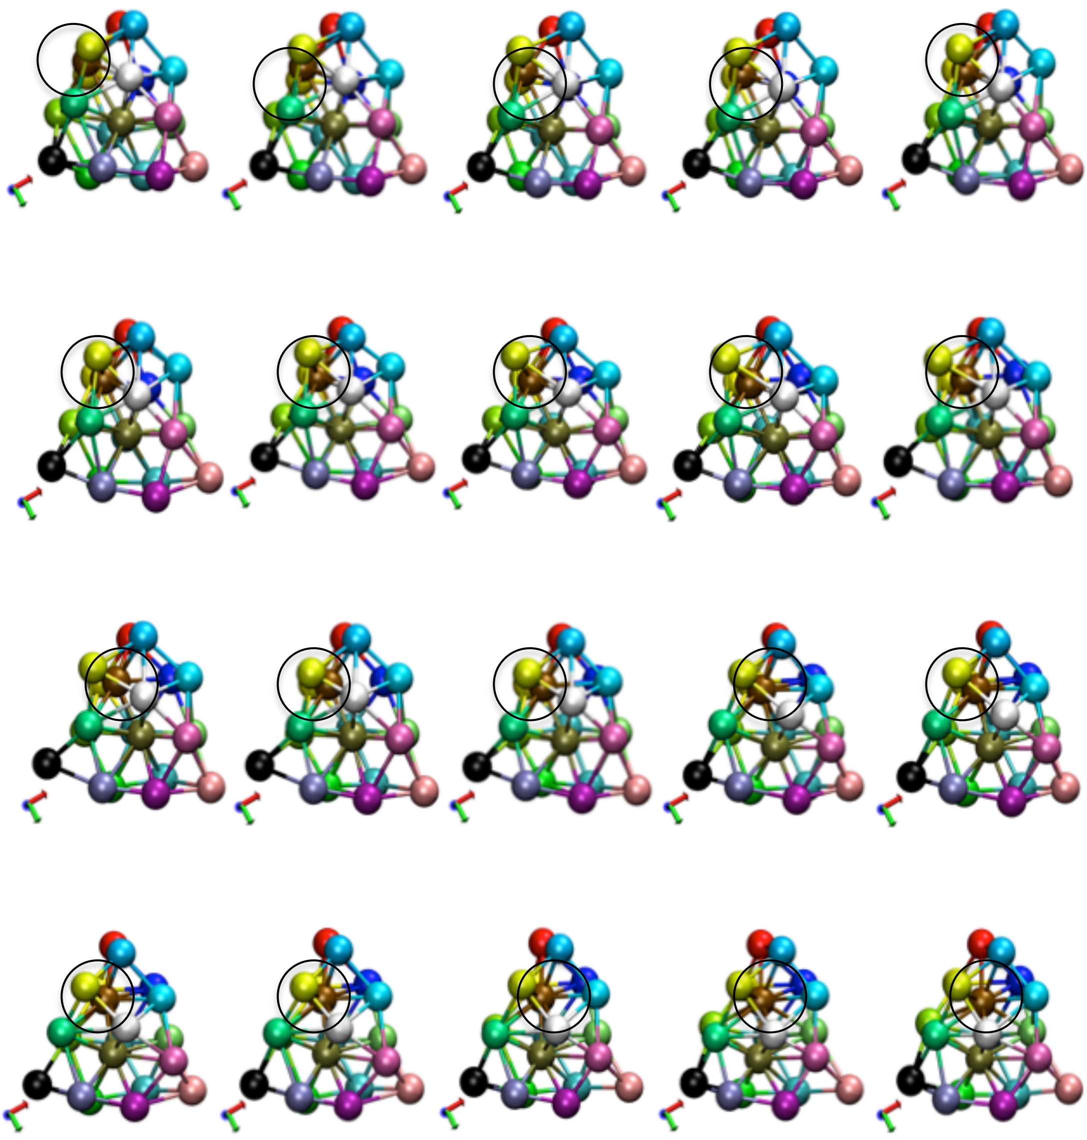

Fig. 5 Twenty consecutive movie steps showing how the surface atom (circled, brown) becomes an internal atom and thus the number of internal atoms changes from one (colored as tan) to two (tan and brown). Note that the overall shape of the cluster does not undergo a significant change.
